# Supplementary material for: Memory-Augmented Reinforcement Learning for Image-Goal Navigation
Source: arXiv:2101.05181 source file (2022-09-12)
Supplement: Supplementary file 1 [file ycviu_supmat.tex]

%% This is file `ycviu-template.tex',
%% 
%% Copyright 2013 Elsevier Ltd
%% 
%% This file is part of the 'Elsarticle Bundle'.
%% ---------------------------------------------
%% 
%% It may be distributed under the conditions of the LaTeX Project Public
%% License, either version 1.2 of this license or (at your option) any
%% later version.  The latest version of this license is in
%%    http://www.latex-project.org/lppl.txt
%% and version 1.2 or later is part of all distributions of LaTeX
%% version 1999/12/01 or later.
%% 
%% The list of all files belonging to the 'Elsarticle Bundle' is
%% given in the file `manifest.txt'.
%% 
%% Template article for Elsevier's document class `elsarticle'
%% with harvard style bibliographic references
%%
%% $Id: ycviu-template-with-authorship.tex 69 2016-07-29 10:15:25Z aptara $
%%
%% This template has no review option
%% 
%% Use the options `twocolumn,final' to obtain the final layout
\documentclass[times,twocolumn,final,authoryear]{elsarticle}

%% Stylefile to load YCVIU template
\usepackage{ycviu}
\usepackage{framed,multirow}

%% The amssymb package provides various useful mathematical symbols
\usepackage{times}
\usepackage{epsfig}
\usepackage{graphicx}
\usepackage{amsmath}
\usepackage{amssymb}
\usepackage{latexsym}

% Following three lines are needed for this document.
% If you are not loading colors or url, then these are
% not required.
\usepackage{url}
\definecolor{newcolor}{rgb}{.8,.349,.1}
\usepackage{booktabs}
\usepackage{multirow}
\usepackage{subcaption}

\usepackage{adjustbox}
\usepackage[utf8]{inputenc}
\usepackage{pifont}
\usepackage{newunicodechar}
\newunicodechar{✓}{\ding{51}}
\newunicodechar{✗}{\ding{55}}
\usepackage[dvipsnames]{xcolor}

\journal{Computer Vision and Image Understanding}

\begin{document}

\thispagestyle{empty}

\ifpreprint
  \setcounter{page}{1}
\else
  \setcounter{page}{1}
\fi

%\begin{frontmatter}

%\title{Memory-Augmented Reinforcement Learning for Image-Goal Navigation - Supplementary Material}

%\end{frontmatter}

%\linenumbers

%% main text
\appendix
\input{supmat}

\bibliographystyle{model2-names}
\bibliography{refs}

\end{document}
